# Supplementary material for: UAV-SEAD: State Estimation Anomaly Dataset for UAVs
Source: arXiv:2602.13900 source file (2026-02-14)
Supplement: Supplementary file 1 [file appendix.tex]

\onecolumn

\appendix
\section{Complete List of PX4 Topics}
\label{app:px4-topics}

% Replace the {lll} with your actual column specifiers.
\begin{longtable}{lll}
  \caption{Full list of topics and their representations of PX4 ULG logging format}
  \label{tab:px4-subtopics}\\

  \toprule
  \textbf{Topic} & \textbf{Subtopics} & \textbf{Representation} \\
  \midrule
  \endfirsthead

  \multicolumn{3}{@{}l}{\textit{(continued)}} \\
  \toprule
  \textbf{Topic} & \textbf{Subtopic} & \textbf{Meaning} \\
  \midrule
  \endhead

  \bottomrule
  \multicolumn{3}{r}{\textit{(continued on next page)}} \\
  \endfoot

  \bottomrule
  \endlastfoot

  %— start of your rows —
  \multirow{9}{*}{actuator\_controls\_0}
    & timestamp\_sample & Timestamp at which the control sample was taken \\
    & control[0]        & Actuator control channel 0 value \\
    & control[1]        & Actuator control channel 1 value \\
    & control[2]        & Actuator control channel 2 value \\
    & control[3]        & Actuator control channel 3 value \\
    & control[4]        & Actuator control channel 4 value \\
    & control[5]        & Actuator control channel 5 value \\
    & control[6]        & Actuator control channel 6 value \\
    & control[7]        & Actuator control channel 7 value \\
  \midrule
  \multirow{17}{*}{actuator\_outputs}
    & noutputs   & Number of actuator outputs \\
    & output[0]  & Output value for actuator channel 0 \\
    & output[1]  & Output value for actuator channel 1 \\
    & output[2]  & Output value for actuator channel 2 \\
    & output[3]  & Output value for actuator channel 3 \\
    & output[4]  & Output value for actuator channel 4 \\
    & output[5]  & Output value for actuator channel 5 \\
    & output[6]  & Output value for actuator channel 6 \\
    & output[7]  & Output value for actuator channel 7 \\
    & output[8]  & Output value for actuator channel 8 \\
    & output[9]  & Output value for actuator channel 9 \\
    & output[10] & Output value for actuator channel 10 \\
    & output[11] & Output value for actuator channel 11 \\
    & output[12] & Output value for actuator channel 12 \\
    & output[13] & Output value for actuator channel 13 \\
    & output[14] & Output value for actuator channel 14 \\
    & output[15] & Output value for actuator channel 15 \\
  \midrule
  \multirow{17}{*}{battery\_status}
    & voltage\_v               & Measured battery voltage (V) \\
    & voltage\_filtered\_v     & Filtered battery voltage (V) \\
    & voltage\_discharged\_mah & Discharged capacity (mAh) \\
    & current\_a               & Measured current (A) \\
    & current\_filtered\_a     & Filtered current (A) \\
    & temperature              & Battery temperature (°C) \\
    & design\_capacity         & Battery design capacity (mAh) \\
    & remaining                & Remaining battery capacity (\%) \\
    & scale                    & Scale factor for capacity \\
    & cell\_id                 & Identifier of battery cell/module \\
    & cycle\_count             & Number of charge/discharge cycles \\
    & connected                & Is battery connected? (1 = yes, 0 = no) \\
    & source                   & Source of battery data \\
    & priority                 & Priority level of this battery \\
    & remaining\_time          & Estimated remaining time (s) \\
    & capacity                 & Current battery capacity (mAh) \\
    & is\_powering\_off        & Indicates imminent power‐off (boolean) \\
    & warning                  & Battery warning level \\
  \midrule
  \multirow{2}{*}{cpuload}
    & load       & CPU utilization (\%) \\
    & ram\_usage & RAM usage (\%) \\
  \midrule
  \multirow{9}{*}{distance\_sensor}
    & min\_distance           & Minimum measurable distance (m) \\
    & max\_distance           & Maximum measurable distance (m) \\
    & current\_distance       & Current measured distance (m) \\
    & signal\_quality         & Quality of sensor signal (integer) \\
    & timestamp               & Time of measurement (μs since boot) \\
    & time\_since\_last\_update & Time since last update (μs) \\
    & type                    & Sensor type identifier \\
    & id                      & Sensor instance ID \\
    & orientation             & Mounting orientation of the sensor \\
  \midrule
  \multirow{10}{*}{ekf2\_innovations}
    & vel\_pos\_innov[0]      & Velocity/position innovation for state 0 \\
    & vel\_pos\_innov[1]      & Velocity/position innovation for state 1 \\
    & vel\_pos\_innov[2]      & Velocity/position innovation for state 2 \\
    & vel\_pos\_innov[3]      & Velocity/position innovation for state 3 \\
    & vel\_pos\_innov[4]      & Velocity/position innovation for state 4 \\
    & vel\_pos\_innov[5]      & Velocity/position innovation for state 5 \\
    & vel\_pos\_innov[6]      & Velocity/position innovation for state 6 \\
    & vel\_pos\_innov[7]      & Velocity/position innovation for state 7 \\
    & aux\_vel\_innov[0]      & Auxiliary velocity innovation for state 0 \\
    & aux\_vel\_innov[1]      & Auxiliary velocity innovation for state 1 \\
  \midrule
  \multirow{10}{*}{estimator\_status}
    & states[0]               & Estimator state flag 0 \\
    & states[1]               & Estimator state flag 1 \\
    & states[2]               & Estimator state flag 2 \\
    & states[3]               & Estimator state flag 3 \\
    & states[4]               & Estimator state flag 4 \\
    & states[5]               & Estimator state flag 5 \\
    & states[6]               & Estimator state flag 6 \\
    & states[7]               & Estimator state flag 7 \\
    & health\_flags           & Health indicator flags of the estimator \\
    & timeout\_flags          & Timeout indicator flags of the estimator \\
  \midrule
  \multirow{20}{*}{input\_rc}
    & timestamp\_last\_signal & Time of last valid RC signal (μs) \\
    & channel\_count          & Number of RC channels received \\
    & channels[0]             & RC channel 0 PWM value \\
    & channels[1]             & RC channel 1 PWM value \\
    & channels[2]             & RC channel 2 PWM value \\
    & channels[3]             & RC channel 3 PWM value \\
    & channels[4]             & RC channel 4 PWM value \\
    & channels[5]             & RC channel 5 PWM value \\
    & channels[6]             & RC channel 6 PWM value \\
    & channels[7]             & RC channel 7 PWM value \\
    & channels[8]             & RC channel 8 PWM value \\
    & channels[9]             & RC channel 9 PWM value \\
    & channels[10]            & RC channel 10 PWM value \\
    & channels[11]            & RC channel 11 PWM value \\
    & channels[12]            & RC channel 12 PWM value \\
    & channels[13]            & RC channel 13 PWM value \\
    & channels[14]            & RC channel 14 PWM value \\
    & channels[15]            & RC channel 15 PWM value \\
    & rssi                    & Received signal strength indicator \\
    & rc\_lost                & RC link lost flag (boolean) \\
    & rc\_failsafe            & RC failsafe activated flag (boolean) \\
    & input\_source           & Source of RC input (e.g., PWM, SBUS) \\
  \midrule
  \multirow{22}{*}{manual\_control\_setpoint}
    & timestamp\_ms           & Time of manual input (ms since boot) \\
    & x                       & Lateral stick input (−1.0 to 1.0) \\
    & y                       & Longitudinal stick input (−1.0 to 1.0) \\
    & z                       & Throttle stick input (0.0 to 1.0) \\
    & r                       & Yaw stick input (−1.0 to 1.0) \\
    & aux1                    & First auxiliary switch/knob value \\
    & aux2                    & Second auxiliary switch/knob value \\
    & aux3                    & Third auxiliary switch/knob value \\
    & aux4                    & Fourth auxiliary switch/knob value \\
    & mode\_switch            & Flight mode switch position \\
    & nav\_mode\_switch       & Navigation mode switch position \\
    & return\_switch          & Return‐to‐home switch position \\
    & rattitude\_switch       & Rattitude mode switch position \\
    & posctl\_switch          & Position control switch position \\
    & loiter\_switch          & Loiter mode switch position \\
    & acro\_switch            & Acro mode switch position \\
    & offboard\_switch        & Offboard mode switch position \\
    & kill\_switch            & Kill switch position \\
    & arm\_switch             & Arm/disarm switch position \\
    & transition\_switch      & VTOL transition switch position \\
    & stab\_switch            & Stabilize mode switch position \\
    & man\_switch             & Manual mode switch position \\
  \midrule
  \multirow{10}{*}{rate\_ctrl\_status}
    & timestamp               & Time of rate control status (μs) \\
    & rollspeed\_rejected     & Indicator if roll rate was rejected \\
    & pitchspeed\_rejected    & Indicator if pitch rate was rejected \\
    & yawspeed\_rejected      & Indicator if yaw rate was rejected \\
    & rollspeed\_integral     & Integral term for roll rate controller \\
    & pitchspeed\_integral    & Integral term for pitch rate controller \\
    & yawspeed\_integral      & Integral term for yaw rate controller \\
    & aux\_integral1          & First auxiliary integral term \\
    & aux\_integral2          & Second auxiliary integral term \\
    & additional\_integral1   & Additional integral term \\
  \midrule
  \multirow{13}{*}{sensor\_combined}
    & timestamp               & Time of combined sensor data (μs) \\
    & gyro\_rad[0]            & Gyroscope X‐axis angular rate (rad/s) \\
    & gyro\_rad[1]            & Gyroscope Y‐axis angular rate (rad/s) \\
    & gyro\_rad[2]            & Gyroscope Z‐axis angular rate (rad/s) \\
    & accelerometer\_m\_s2[0] & Accelerometer X‐axis (m/s²) \\
    & accelerometer\_m\_s2[1] & Accelerometer Y‐axis (m/s²) \\
    & accelerometer\_m\_s2[2] & Accelerometer Z‐axis (m/s²) \\
    & adc\_voltages[0]        & ADC voltage input channel 0 \\
    & adc\_voltages[1]        & ADC voltage input channel 1 \\
    & adc\_voltages[2]        & ADC voltage input channel 2 \\
    & adc\_voltages[3]        & ADC voltage input channel 3 \\
    & adc\_voltages[4]        & ADC voltage input channel 4 \\
    & accelerometer\_integral\_dt & Time interval for accelerometer integration (μs) \\
  \midrule
  \multirow{4}{*}{sensor\_preflight}
    & timestamp               & Time of preflight sensor check (μs) \\
    & accel\_inconsistency\_m\_s2 & Accelerometer inconsistency (m/s²) \\
    & gyro\_inconsistency\_rad\_s  & Gyroscope inconsistency (rad/s) \\
    & mag\_inconsistency\_angle    & Magnetometer inconsistency (rad) \\
  \midrule
  \multirow{14}{*}{system\_power}
    & timestamp               & Time of power status (μs) \\
    & voltage5v\_v            & 5V rail voltage (V) \\
    & voltage3v3\_v           & 3.3V rail voltage (V) \\
    & voltage\_battery\_v     & Battery voltage (V) \\
    & current\_battery\_a     & Battery current draw (A) \\
    & current\_usb\_a         & USB current draw (A) \\
    & current\_servo\_rail\_a & Servo rail current draw (A) \\
    & current\_periph\_rail\_a& Peripheral rail current draw (A) \\
    & v5\_oc\_circuit         & 5V over-current circuit status \\
    & v5\_oc\_pwm             & 5V over-current PWM status \\
    & flash\_fail             & Flash memory failure indicator \\
    & usb\_current\_a         & USB current (A) \\
    & periph\_5v\_oc          & Peripheral 5V over-current indicator \\
    & hipower\_5v\_oc         & High-power 5V over-current indicator \\
  \midrule
  \multirow{16}{*}{telemetry\_status}
    & timestamp               & Time of telemetry status (μs) \\
    & heartbeat\_time         & Time of last heartbeat (μs) \\
    & status                  & Overall telemetry status code \\
    & type                    & Telemetry link type identifier \\
    & rate\_tx                & Telemetry transmission rate (bytes/s) \\
    & rate\_txerr             & Telemetry transmit errors count \\
    & rate\_txe\_mavlink1     & MAVLink v1 transmit errors count \\
    & rate\_txe\_mavlink2     & MAVLink v2 transmit errors count \\
    & rate\_txe\_uorb         & uORB transmit errors count \\
    & rate\_txe\_buffer       & Buffer transmit errors count \\
    & rate\_txe\_fail         & Total transmit failures \\
    & rate\_txe\_overflow     & Transmit buffer overflow count \\
    & streams                 & Number of active telemetry streams \\
    & ftp                     & FTP status (enabled/disabled) \\
    & mavlink\_v2             & MAVLink v2 status (enabled/disabled) \\
  \midrule
  \multirow{1}{*}{timestamp}
    & timestamp               & System-wide timestamp (μs since boot) \\
  \midrule
  \multirow{8}{*}{vehicle\_air\_data}
    & timestamp               & Time of air data (μs) \\
    & baro\_alt\_meter        & Barometric altitude (m) \\
    & baro\_pressure\_pa      & Barometric pressure (Pa) \\
    & baro\_temperature\_deg\_c & Barometric temperature (°C) \\
    & airspeed\_m\_s          & Measured airspeed (m/s) \\
    & true\_airspeed\_m\_s    & True airspeed (m/s) \\
    & density\_air\_kg\_m3     & Air density (kg/m³) \\
    & rho                     & Air density ratio parameter \\
  \midrule
  \multirow{4}{*}{vehicle\_angular\_velocity}
    & timestamp               & Time of angular velocity data (μs) \\
    & xyz[0]                  & Angular velocity around X-axis (rad/s) \\
    & xyz[1]                  & Angular velocity around Y-axis (rad/s) \\
    & xyz[2]                  & Angular velocity around Z-axis (rad/s) \\
  \midrule
  \multirow{10}{*}{vehicle\_attitude}
    & timestamp               & Time of attitude estimate (μs) \\
    & q[0]                    & Quaternion component w \\
    & q[1]                    & Quaternion component x \\
    & q[2]                    & Quaternion component y \\
    & q[3]                    & Quaternion component z \\
    & delta\_q\_reset[0]      & Quaternion reset delta component w \\
    & delta\_q\_reset[1]      & Quaternion reset delta component x \\
    & delta\_q\_reset[2]      & Quaternion reset delta component y \\
    & delta\_q\_reset[3]      & Quaternion reset delta component z \\
    & quat\_reset\_counter    & Number of quaternion resets \\
  \midrule
  \multirow{13}{*}{vehicle\_attitude\_setpoint}
    & roll\_body              & Desired roll angle (rad) \\
    & pitch\_body             & Desired pitch angle (rad) \\
    & yaw\_body               & Desired yaw angle (rad) \\
    & thrust\_body[0]         & Desired thrust X component \\
    & thrust\_body[1]         & Desired thrust Y component \\
    & thrust\_body[2]         & Desired thrust Z component \\
    & q\_d[0]                 & Desired quaternion component w \\
    & q\_d[1]                 & Desired quaternion component x \\
    & q\_d[2]                 & Desired quaternion component y \\
    & q\_d[3]                 & Desired quaternion component z \\
    & yaw\_feedforward         & Yaw feedforward term \\
    & fw\_control\_yaw         & Fixed-wing control yaw term \\
    & apply\_flaps             & Flaps deployment flag \\
  \midrule
  \multirow{4}{*}{vehicle\_land\_detected}
    & timestamp               & Time of land detection (μs) \\
    & alt\_max                & Maximum altitude for land detection (m) \\
    & landed                  & Landed status (boolean) \\
    & in\_ground\_effect      & In ground effect status (boolean) \\
  \midrule
  \multirow{5}{*}{vehicle\_local\_position}
    & timestamp               & Time of local position data (μs) \\
    & ref\_timestamp          & Reference timestamp for position (μs) \\
    & xy\_global              & Global XY position (degrees) \\
    & z\_global               & Global altitude (m) \\
    & dist\_bottom\_valid     & Validity of bottom distance data (boolean) \\
  \midrule
  \multirow{4}{*}{vehicle\_magnetometer}
    & timestamp               & Time of magnetometer data (μs) \\
    & magnetometer\_ga[0]     & Magnetic field X component (G) \\
    & magnetometer\_ga[1]     & Magnetic field Y component (G) \\
    & magnetometer\_ga[2]     & Magnetic field Z component (G) \\
  \midrule
  \multirow{6}{*}{vehicle\_rates\_setpoint}
    & roll                    & Desired roll rate (rad/s) \\
    & pitch                   & Desired pitch rate (rad/s) \\
    & yaw                     & Desired yaw rate (rad/s) \\
    & thrust\_body[0]         & Desired thrust X component \\
    & thrust\_body[1]         & Desired thrust Y component \\
    & thrust\_body[2]         & Desired thrust Z component \\
  \midrule
  \multirow{2}{*}{vehicle\_status}
    & timestamp               & Time of vehicle status (μs) \\
    & onboard\_control\_sensors\_present & Bitmask of onboard sensors present \\
    & onboard\_control\_sensors\_enabled & Bitmask of onboard sensors enabled \\
    & onboard\_control\_sensors\_health  & Bitmask of onboard sensors health \\
    & rtc\_failing            & RTC failing indicator (boolean) \\
    & calibration\_enabled    & Calibration status (boolean) \\
    & mission\_failure\_status & Mission failure code \\
    & condition\_calibration\_enabled  & Calibration condition flag \\
    & condition\_horizontal\_position\_valid & Horizontal position validity \\
    & condition\_local\_altitude\_valid  & Local altitude validity \\
    & condition\_global\_position\_valid & Global position validity \\
    & condition\_local\_velocity\_valid  & Local velocity validity \\
    & condition\_angular\_velocity\_valid & Angular velocity validity \\
    & condition\_attitude\_valid & Attitude validity flag \\
    & condition\_battery\_ok    & Battery OK condition (boolean) \\
    & condition\_home\_position\_valid & Home position validity \\
    & condition\_system\_ready  & System readiness flag \\
    & condition\_auto\_mission\_available & Auto mission available flag \\
    & condition\_yaw\_valid     & Yaw validity flag \\
    & condition\_gps\_fixed     & GPS fix status (boolean) \\
    & condition\_indoor\_usable & Indoor usability status \\
    & condition\_power\_input\_valid & Power input validity flag \\
    & condition\_gps\_glitch\_imminent & GPS glitch imminent (boolean) \\
    & condition\_accelerometer\_healthy & Accelerometer health (boolean) \\
    & condition\_gyroscope\_healthy    & Gyroscope health (boolean) \\
    & condition\_magnetometer\_healthy & Magnetometer health (boolean) \\
    & condition\_barometer\_healthy    & Barometer health (boolean) \\
    & condition\_optical\_flow\_healthy & Optical flow sensor health (boolean) \\
    & condition\_distance\_sensor\_healthy & Distance sensor health (boolean) \\
    & condition\_landing\_sensor\_valid & Landing sensor validity (boolean) \\
    & condition\_airspeed\_valid      & Airspeed validity (boolean) \\
    & condition\_rev\_condition       & Reserved condition flag \\
    & condition\_circuit\_breaker\_engaged & Circuit breaker engaged (boolean) \\
    & condition\_vtol\_in\_transition & VTOL in transition (boolean) \\
    & condition\_vtol\_FW\_in\_transition & Fixed-wing VTOL in transition (boolean) \\
    & aspd\_use\_inhibit              & Airspeed inhibit flag (boolean) \\
    & aspd\_fail\_rtl                 & Airspeed failure in RTL (boolean) \\
  \midrule
  \multirow{11}{*}{vehicle\_status\_flags}
    & timestamp               & Time of status flags (μs) \\
    & condition\_calibration\_enabled   & Calibration condition flag \\
    & condition\_horizontal\_position\_valid & Horizontal position validity \\
    & condition\_local\_altitude\_valid  & Local altitude validity \\
    & condition\_global\_position\_valid & Global position validity \\
    & condition\_local\_velocity\_valid  & Local velocity validity \\
    & condition\_angular\_velocity\_valid & Angular velocity validity \\
    & condition\_attitude\_valid & Attitude validity flag \\
    & condition\_battery\_ok    & Battery OK condition \\
    & condition\_home\_position\_valid & Home position validity \\
    & condition\_system\_required & System required flag (boolean) \\
    & avoidance\_system\_valid  & Collision avoidance system validity \\
  %— end of your rows —
\end{longtable}
